# Supplementary material for: Information Flows in Encrypted Databases
Source: arXiv:1605.01092 source file (2016-05-03)
Supplement: Supplementary file 1 [file appendix.tex]

\section{Semantic Equivalence}
\label{sec:equivalence}
An execution of the application \app{} can be represented as a \textit{history} \history{}.
A history is a sequence of \textit{call} and \textit{return} events.
A call event \callproc\ represents a call to a stored procedure with parameters \param. 
A return event \returnproc\ represents control returning from the stored procedure. 
A history is \textit{complete} is every call has a matching return event.
Histories may be \textit{concurrent} -- a history is concurrent if some prefix of the history has multiple call events without a matching return event. 
We say that a history \history{} is generated from a configuration \config{} if there exists an execution where \database{} is the initial state of the database, and calls are made to procedures in \app{}.

Let $\history{}[i]$ represent the $i^{th}$ event in the history \history{}. 
Two histories \history{} and \history{'} are \textit{identical} every event $\history{}[i]$ is identical to $\history{'}[i]$. 
Note histories generated from different configurations can be identical.
For example, if stored procedures in an application \app{} are refactored or optimized without changing semantics, or an index is added to a database, the resulting configuration can generate identical histories. 

We say that two configurations \config{1} and \config{2} are \textit{semantically equivalent} if for every history \history{} generated from \config{1}, there exists an identical history \history{'} generated from \config{2} and vice versa.
An example of semantically equivalent configurations arises in the context of encryption. 
If we encrypt some columns of the database, and rewrite the application by introducing calls to encryption and decryption routines at the appropriate program points, we can obtain two semantically equivalent configurations. 
Formally, 

\begin{definition}
\label{def:semantics-preserving}
Let \database{\policy} represent the database obtained by encrypting all columns in \database{} according to the policy \policy. 
Consider an application \app{}, and another application \app{\policy} obtained by rewriting \app{}.
We say that such a rewriting is \textit{semantics preserving} if the configurations \config{} and (\app{\policy},\database{\policy}) are semantically equivalent. 
\end{definition}
